# Supplementary material for: Test-Time Optimization for Domain Adaptive Open Vocabulary Segmentation
Source: arXiv:2501.04696 source file (2025-03-08)
Supplement: Supplementary file 1 [file additional_ablation_attr_aggre.tex]

\begin{minipage}{0.15\textwidth}  % 0.48
\centering
\small
  % height
\setlength\tabcolsep{0.7em}  % width
\scalebox{0.85}{  % 0.95
\begin{tabular}{ll|c}
\toprule
& Method & DZ \\ \midrule
\rowcolor{Gray}
\textbf{(I)}   & Our final method   & 34.6 \\
\textbf{(II)}  & \textbf{(I)} - WA  & 33.3 \\
\textbf{(III)} & \textbf{(I)} - NAE  & 33.3 \\
\textbf{(IV)}  & \textbf{(I)} - NCE  & 33.3 \\
\textbf{(V)}   & \textbf{(I)} - NAE \& NCE  & 33.3 \\
\bottomrule
\end{tabular}
}
% \vspace{-1.0em}
\caption{\footnotesize
\textbf{Additional Ablation - Attribute Aggregation}: We report mIoU on Dark Zurich (DZ) \cite{sakaridis2019guided} dataset.
}
\label{tbl:addi_attr_aggregation}
\end{minipage}
